# Supplementary material for: Lower Bounds on Cross-Entropy Loss in the Presence of Test-time Adversaries
Source: arXiv:2104.08382 source file (2021-06-04)
Supplement: Supplementary file 1 [file appendix.tex]

\section{Proofs for lower bound on mixture of Gaussians}
\todo{later!}

\section{Proofs for Algorithm 1}

\begin{lemma}
\label{lemma: linopt-props}
  The function $\textsf{LinOpt}(\mcA,\mcB,\mcE,P)$ produces $(\mcA^+,\mcA^-,\mcB^+,\mcB^-,z)$ with the following properties.
  \begin{outline}[enumerate]
      \1 $P(\mcA^+)P(\mcB^+) \geq P(\mcA^-)P(\mcB^-)$
%      \item If $P(\mcA^+)P(\mcB^+) > P(\mcA^-)P(\mcB^-)$, then all of $\mcA^+,\mcA^-,\mcB^+,\mcB^-$ are nonempty (This is not true if we allow isolated vertices, and the plus sets are nonempty because they have positive probability
      \1 If $P(\mcA^+)P(\mcB^+) = P(\mcA^-)P(\mcB^-)$, then
      \2 $\one^{\top}z = P(\mcA \cup \mcB)$, 
      \2$\frac{P(\mcA)}{P(\mcA \cup \mcB)}(M^{\top} z)_v = P(\{v\})$ for all $v \in \mcA$, 
      \2$\frac{P(\mcB)}{P(\mcA \cup \mcB)}(M^{\top} z)_v = P(\{v\})$ for all $v \in \mcB$.
  \end{outline}
  %will either provide $z$ such that $M^{\top} z = r$ and $\one^{\top} z = r^{\top} \one_{\mcV_+} = r^{\top} \one_{\mcV_-} = \one^{\top} p$, 
  %or a partition $\mcV = \mcU_+ \sqcup \mcU_-$ with the following properties:
%\begin{align*}
  %(\one^{\top}_{\mcV_+ \cap \mcU_+} p) (\one^{\top}_{\mcV_- \cap \mcU_-} p) > (\one^{\top}_{\mcV_+ \cap \mcU_-} p) (\one^{\top}_{\mcV_- \cap \mcU_+} p)
%\end{align*}
\end{lemma}
\begin{proof}
Because each edge contains exactly one vertex in each of $\mcA$ and $\mcB$, $M \one_{\mcA} = \one_{\mcE \cup \mcA}$ and $M \one_{\mcB} = \one_{\mcE \cup \mcB}$.
This gives two feasible choices for $y$: $y = \one_{\mcA}$ and $y = \one_{\mcB}$.
By construction of $r$, at least one of these achieves a value of $P(\mcA \cup \mcB)$.
If $P(\mcA)>0$ then
%Let $a_c = \one_{\mcV_{c}}^{\top}p$.
\[
  r^{\top}\one_{\mcA} = \sum_{v \in \mcA} \frac{P(\mcA \cup \mcB)}{P(\mcA)} p_v =  P(\mcA \cup \mcB)
\]
and if $P(\mcB)>0$ then $r^{\top}\one_{\mcB} = P(\mcA \cup \mcB)$.
Complementary slackness implies $(M^{\top}z - r)^{\top}y = 0$ for all optimal $y$,
and thus $(M^{\top}z - r)_v = 0$ for all $v$ that are nonzero in some optimal $y$.
If the feasible points $y = \one_{\mcA}$ and $y = \one_{\mcB}$ are optimal, then $(M^{\top} z)_v = r_v$ for all $v \in \mcA$ if $P(\mcA) > 0$ and for all $v \in \mcB$ if $P(\mcB) > 0$.
Then Property 2 follows from the definition of $r$.

By strong linear programming duality, we always find $z$ and $y$ such that $\one^{\top} z = r^{\top} y$.
If the candidate choices of $y$ described above are optimal, we satisfy the first alternative of the claim.
Otherwise, we have $y$ such that $r^{\top} y > \one^{\top} p$.
We have
\begin{align*}
  r^{\top}(\one_{\mcA_+} + \one_{\mcB_+}) &> \one^{\top} p\\ 
  \frac{P(\mcA \cup \mcB)P(\mcA^+)}{P(\mcA)} + \frac{P(\mcA \cup \mcB)P(\mcB^+)}{P(\mcB)} &>  P(\mcA \cup \mcB)\\
  P(\mcA^+)P(\mcB)+P(\mcB^+)P(\mcA) &> P(\mcA)P(\mcB)\\
  P(\mcA^+)P(\mcB^+) &> P(\mcA^-)P(\mcB^-)
\end{align*}
which establishes Property 1.
\end{proof}

\begin{lemma}
\label{lemma: optprob-props}
If $P(\mcA \cup \mcB) > 0$, the computation of $\textsf{OptProb}(\mcA,\mcB,\mcE,P)$ terminates and produces a pair $(q,z)$.
For some $[k] = \{0,1,\ldots,k-1\}$, there are functions $a : \mcA \to [k]$ and $b: \mcB \to [k]$ with the following properties.
\begin{outline}[enumerate]
\1 If $(u,v) \in \mcE$, $a(u) \leq b(v)$.
\1 We have $z \geq 0$, $\one^{\top}z = P(\mcA \cup \mcB)$, and $P(\{v\}) = q_v (M^{\top}z)_v$.
%If $z_{(u,v)} > 0$,  then $a(u) = b(v)$. If $z_u > 0$, then $q_u = 1$.
%$a(u) = k-1$. 
%If $z_v > 0$, then $q_v = 1$.
%$b(v) = 0$.
\1 Let $\mcA_{i} = a^{-1}(i)$ and $\mcB_{i} = b^{-1}(i)$.\\
For all $i$, $P(\mcA_{i} \cup \mcB_{i}) > 0$.
For all $u \in \mcA$ and $v \in \mcB$, 
$q_u = \frac{P(\mcA_{a(u)})}{P(\mcA_{a(u)} \cup \mcB_{a(u)})}$ and
$q_v = \frac{P(\mcA_{b(v)})}{P(\mcA_{b(v)} \cup \mcB_{b(v)})}$.

\1 For $u,u' \in \mcA$, if $a(u) \leq a(u')$ then $q_u \leq q_{u'}$.
%\item If $b(v) \leq b(v')$, $q_v \leq q_{v'}$.
\end{outline}
\end{lemma}
%For all $i$,If $a(u) = b(v)$, then $q_u + q_v = 1$. 
%The fact that $a$ and $b$ are surjective along with second property implies that $q$ is constant on each part of the partitions of $\mcA$ and $\mcB$ induced by $a$ and $b$.

\begin{proof}
In the base case of the induction, the output of $\textsf{OptProb}$ comes from the second branch, the computation terminates, and $P(\mcA^+)P(\mcB^+) \leq P(\mcA^-)P(\mcB^-)$.
We take $k=1$, so $\mcA = \mcA_0$ and $\mcB = \mcB_0$.
From Property 1 of Lemma~\ref{lemma: linopt-props}, $P(\mcA^+)P(\mcB^+) = P(\mcA^-)P(\mcB^-)$ and thus from Property 2a we have $\one^{\top}z = P(\mcA \cup \mcB)$
Then $q$ is specified by Line \ref{q-base-case} and satisfies Property 3 by construction.
Properties 2b and 2c of Lemma~\ref{lemma: linopt-props} implies $q_v(M^{\top} z)_v = P(\{v\})$, so Property 2 is established.
Properties 1 and 4 hold trivially when $k=1$.

In the inductive case, the output of $\textsf{OptProb}$ comes from the first branch.
Because $P(\mcA^+)P(\mcB^+) > 0$, both $\mcA^+$ and $\mcB^+$ are nonempty.
Thus $|\mcA^+ \cup \mcB^-| < |\mcA \cup \mcB|$ and $|\mcA^- \cup \mcB^+| < |\mcA \cup \mcB|$, so the recursive calls both involve strictly smaller vertex sets.
By induction, both recursive calls terminate.
Suppose that $(q',z')$ and $(q'',z'')$ satisfy the four properties with functions $a' : \mcA^+ \to [k']$ and $b' : \mcB^- \to [k']$ and $a'' : \mcA^- \to [k'']$ and $b'' : \mcB^+ \to [k'']$ respectively.
Then we take $k = k'+k''$ and define $a$ and $b$ in the following piecewise fashion:
\begin{align*}
a(u) &= \begin{cases}
a'(u)+k'' & u \in \mcA^+\\
a''(u) & u \in \mcA^-\\
\end{cases}\\
b(u) &= \begin{cases}
b'(u)+k'' & u \in \mcB^-\\
b''(u) & u \in \mcB^+\\
\end{cases}
\end{align*}
Because $\mcA^+ \cup \mcB^+$ is an independent set, there are no edges $(u,v)$ with $a(u) \geq k'' > b(v)$.
Along with the induction hypotheses, this established Property 1.
The piecewise definitions of $q$ in line 7 and $z$ in line 8 satisfy Properties 2 and 3 because $(q',z')$ and $(q'',z'')$ do.

Property 4 requires a bit of calculation.
The set $\mcA^+ \cup \mcA_{k''-1} \cup (\mcB^+ \setminus \mcB_{k''-1})$ is an independent set and from the properties of $\textsf{LinOpt}$
\begin{multline*}
P(\mcB)P(\mcA^+) + P(\mcA)P(\mcB^+) \geq\\ P(\mcB)(P(\mcA^+) + P(\mcA_{k''-1})) + P(\mcA)(P(\mcB^+) - P(\mcB_{k''-1}))
\end{multline*}  
so $P(\mcA)P(\mcB_{k''-1}) \geq P(\mcB)P(\mcA_{k''-1})$.
Similarly, $(\mcA^+ \setminus \mcA_{k''}) \cup \mcB^+ \cup \mcB_{k''}$ is an independent set and 
\begin{multline*}
P(\mcB)P(\mcA^+) + P(\mcA)P(\mcB^+) \geq\\ P(\mcB)(P(\mcA^+) - P(\mcA_{k''})) + P(\mcA)(P(\mcB^+) + P(\mcB_{k''}))
\end{multline*}  
so $P(\mcA)P(\mcB_{k''}) \leq P(\mcB)P(\mcA_{k''})$.
Combining these inequalities, we have 
\[
\frac{P(\mcA_{k''-1})}{P(\mcA_{k''-1} \cup \mcB_{k''-1})} \leq 
\frac{P(\mcA)}{P(\mcA \cup \mcB)} \leq
\frac{P(\mcA_{k''})}{P(\mcA_{k''} \cup \mcB_{k''})}.
\]
Along with the induction hypotheses, this establishes Property 4.
\end{proof}

\section{Additional Results}

\subsection{Other class pairs}

\subsection{Graph properties}
- Intersection prob.

\subsection{Runtime analysis for other datasets}

\subsection{$0-1$ loss}
 We note that the optimal classifier probabilities that are obtained in the course of determining the minimum log-loss can be thresholded to obtain the classification outcomes of the optimal classifier. Care must be taken, however, for data points where the optimal probability is $\frac{1}{2}$ in the two class case. For all points of this type, we just classify them as being in class $1$, which avoids any conflicts and recovers the numerical values from previous work \cite{bhagoji2019lower}. These bounds are in \todo{xx} of the Supp..

 \begin{figure}[t]
	\centering
	\subfloat[MNIST]{\resizebox{0.48\textwidth}{!}{\input{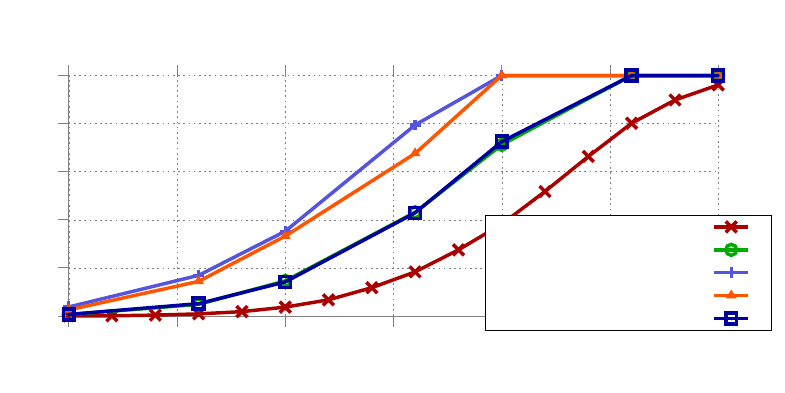}}\label{subfig: mnist_KL}}
	\hspace{0mm}
	\subfloat[Fashion MNIST]{\resizebox{0.48\textwidth}{!}{\input{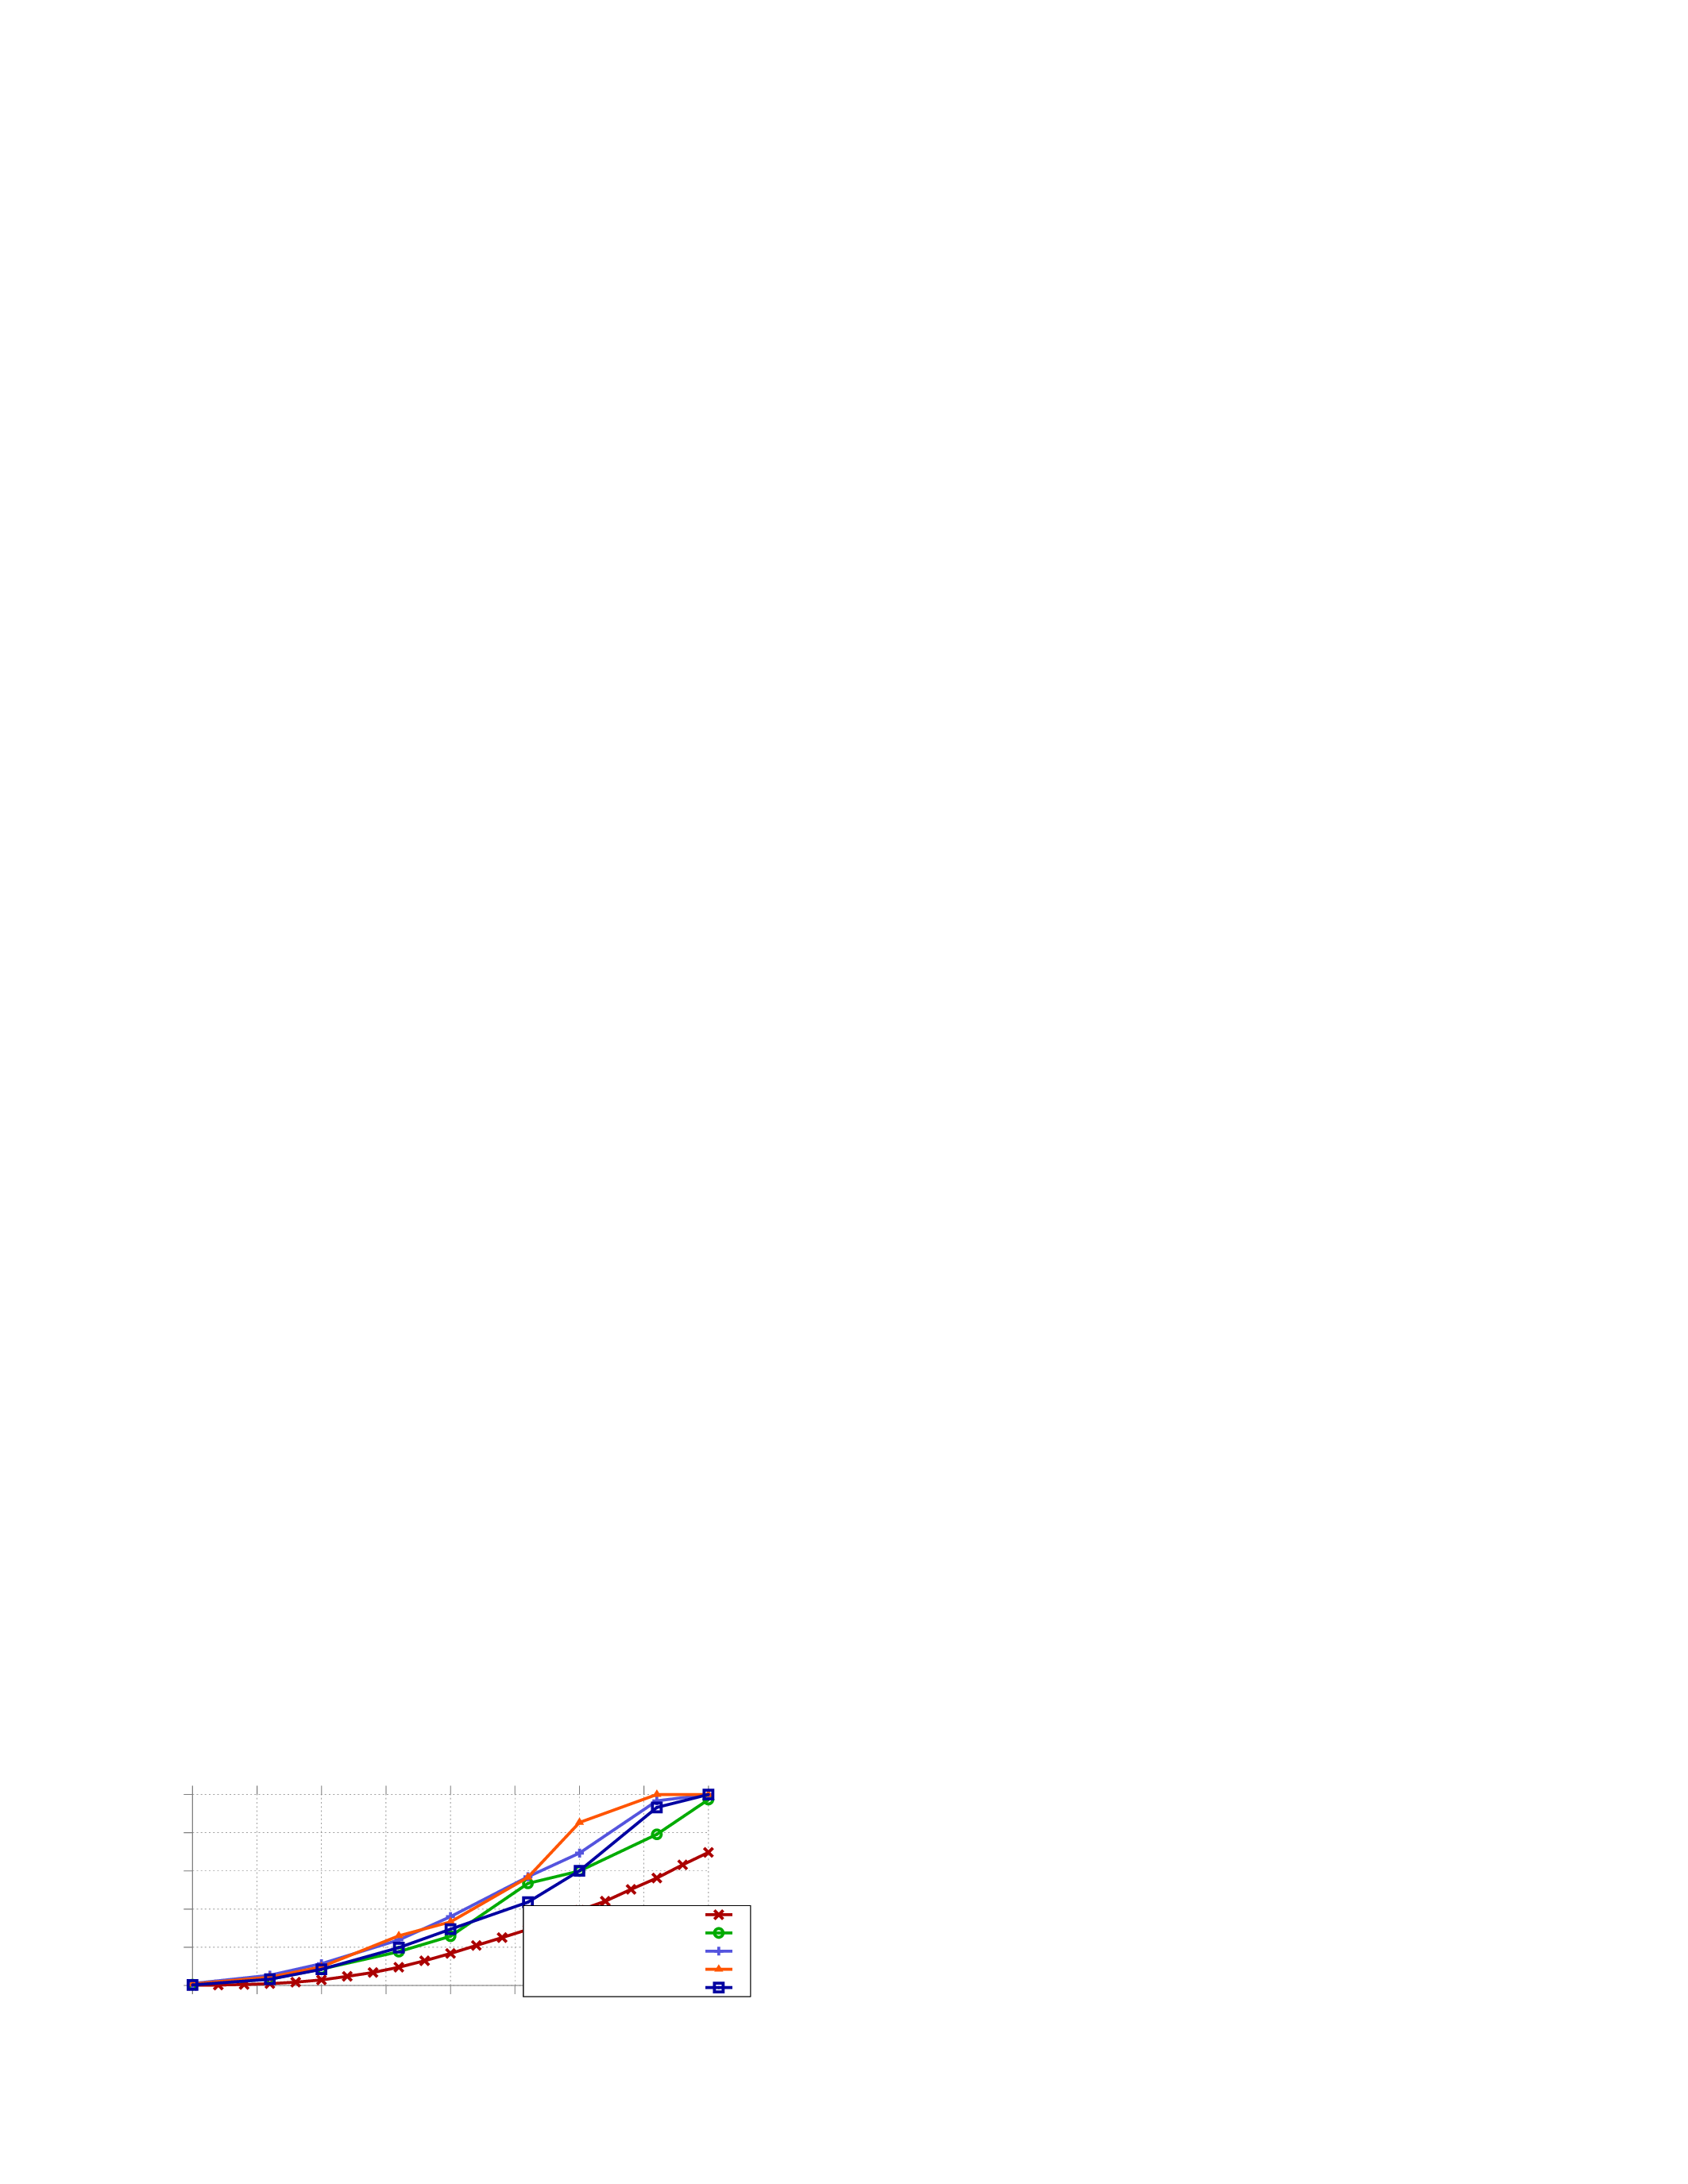}}\label{subfig: fmnist_KL}}
	\caption{Comparison on \emph{training data} between the $0-1$ loss obtained by different training methods (computed using AutoAttack) versus the optimal loss.}
	\label{fig: compare_plot_01}
	\vspace{-10pt}
\end{figure}

\begin{figure}[t]
	\centering
	\subfloat[MNIST]{\resizebox{0.48\textwidth}{!}{\input{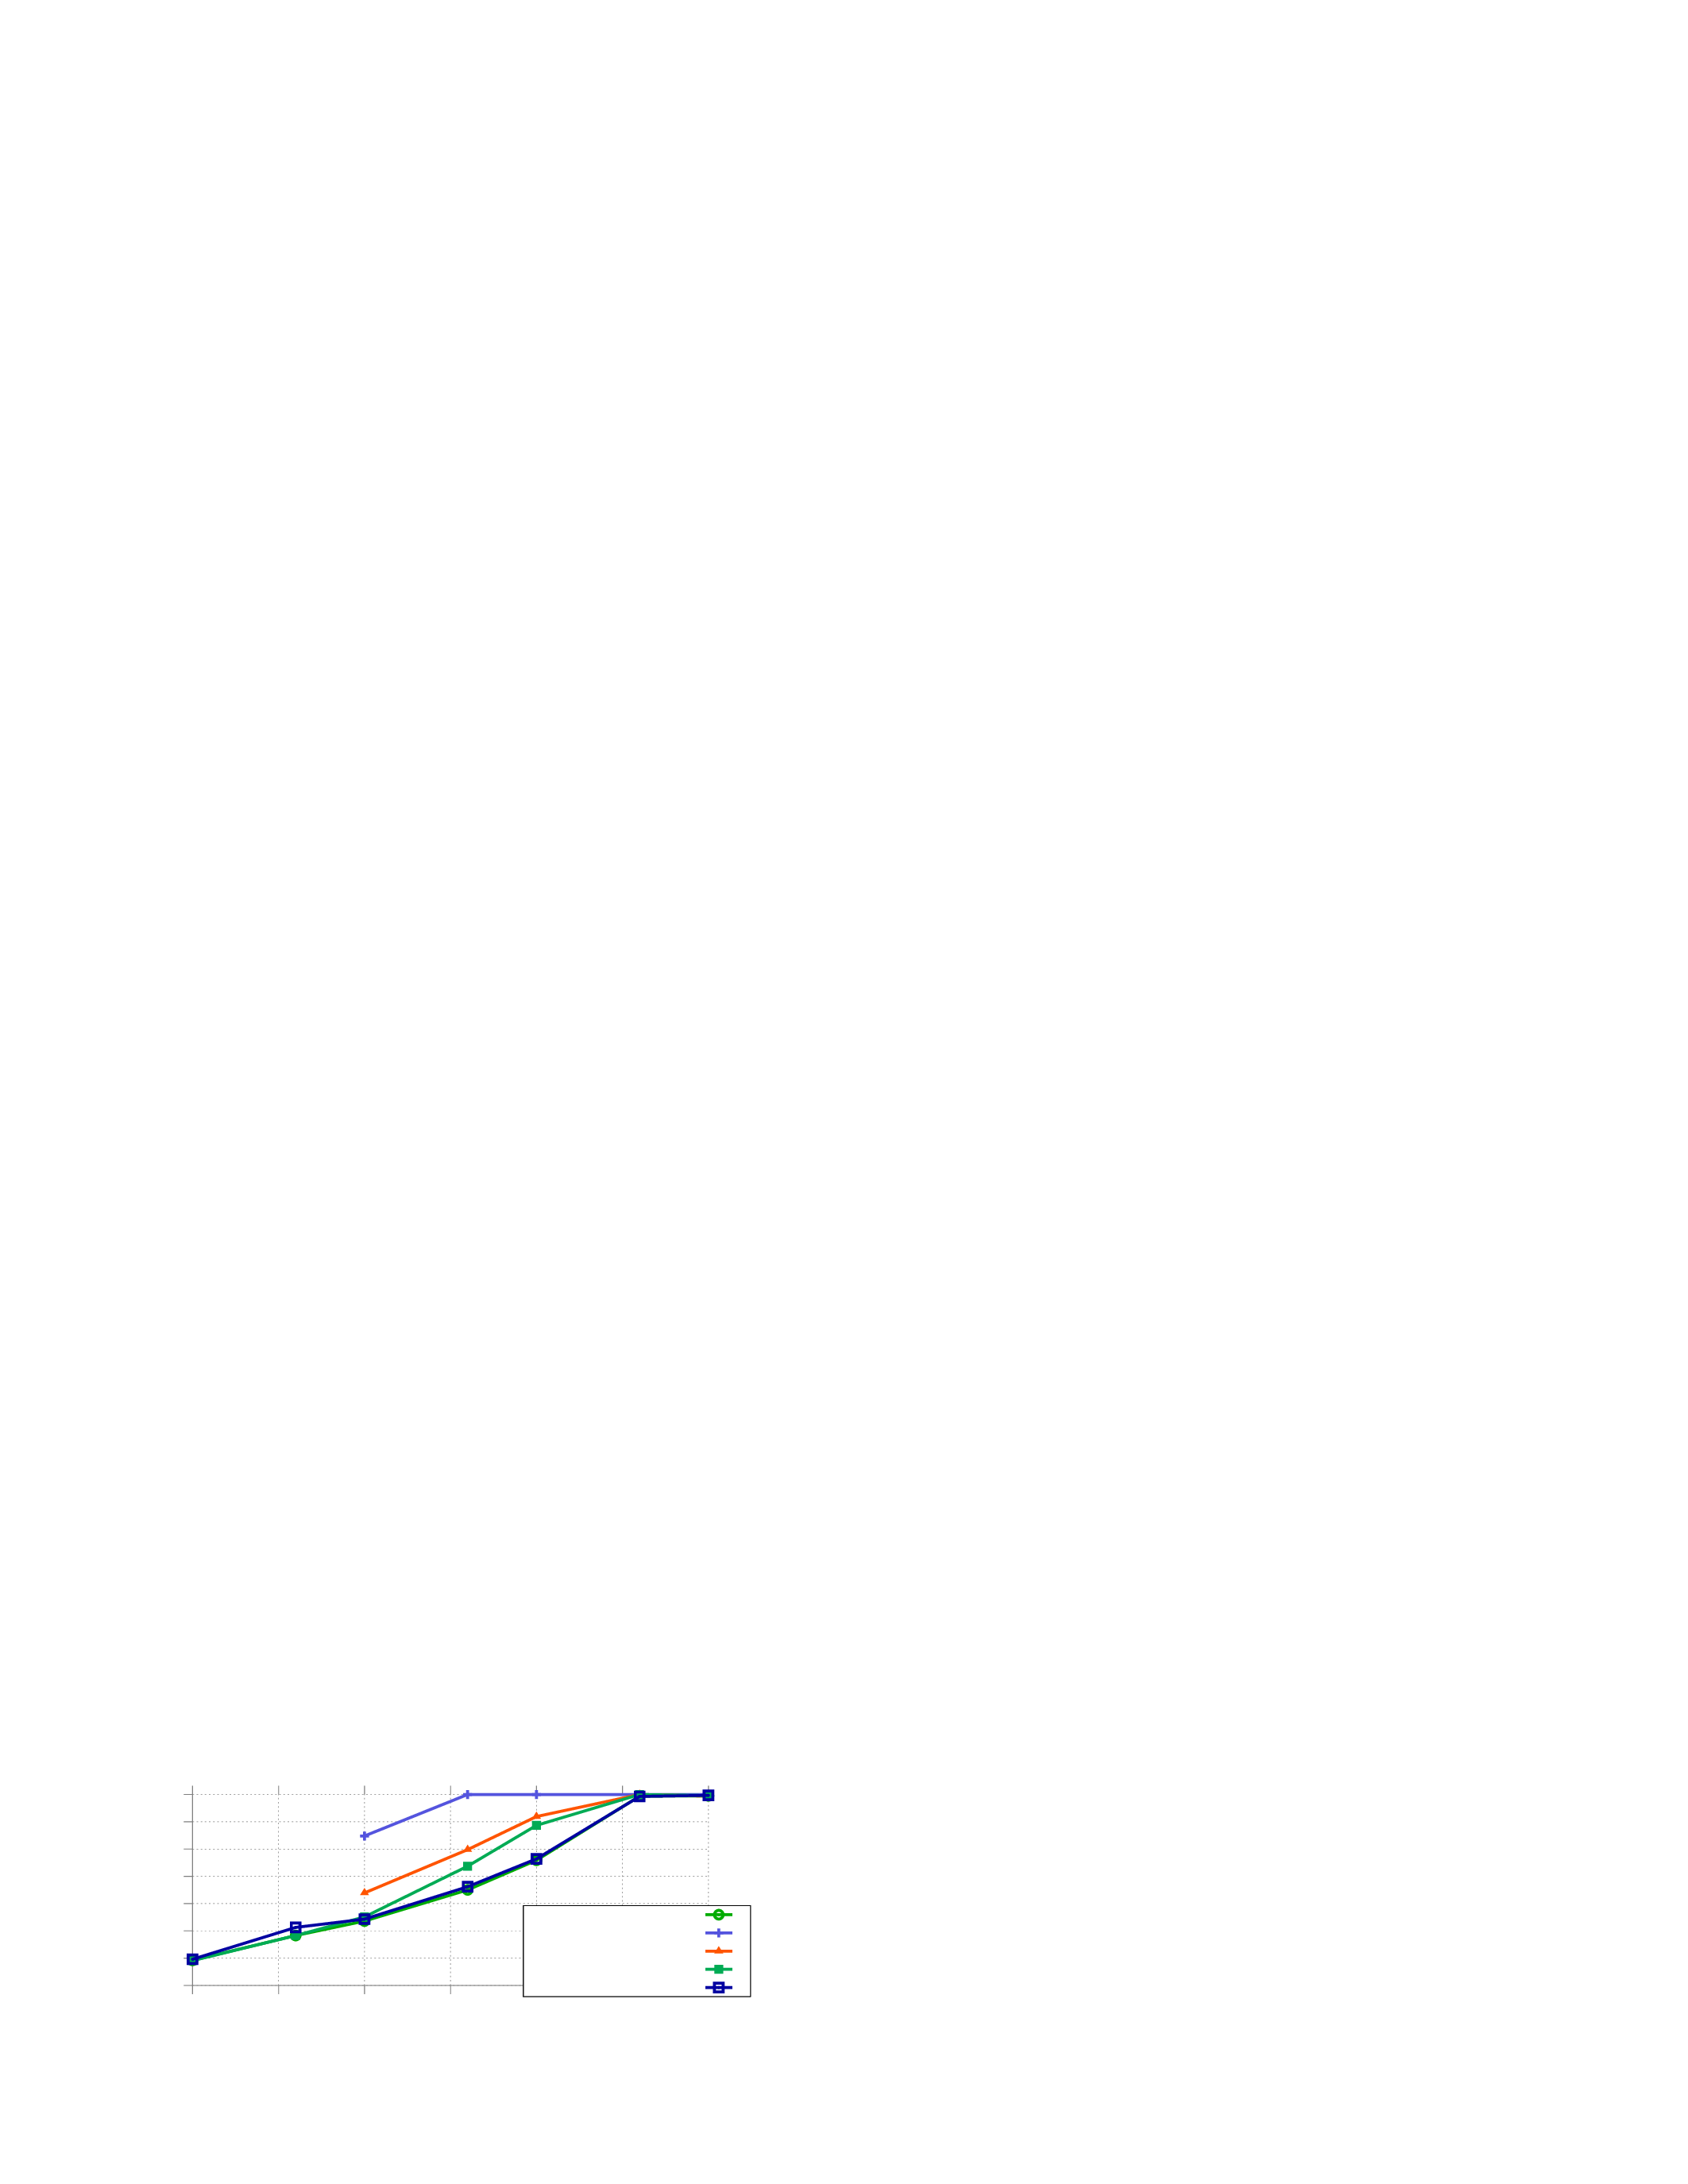}}\label{subfig: mnist_KL_test}}
	\hspace{0mm}
	\subfloat[Fashion MNIST]{\resizebox{0.48\textwidth}{!}{\input{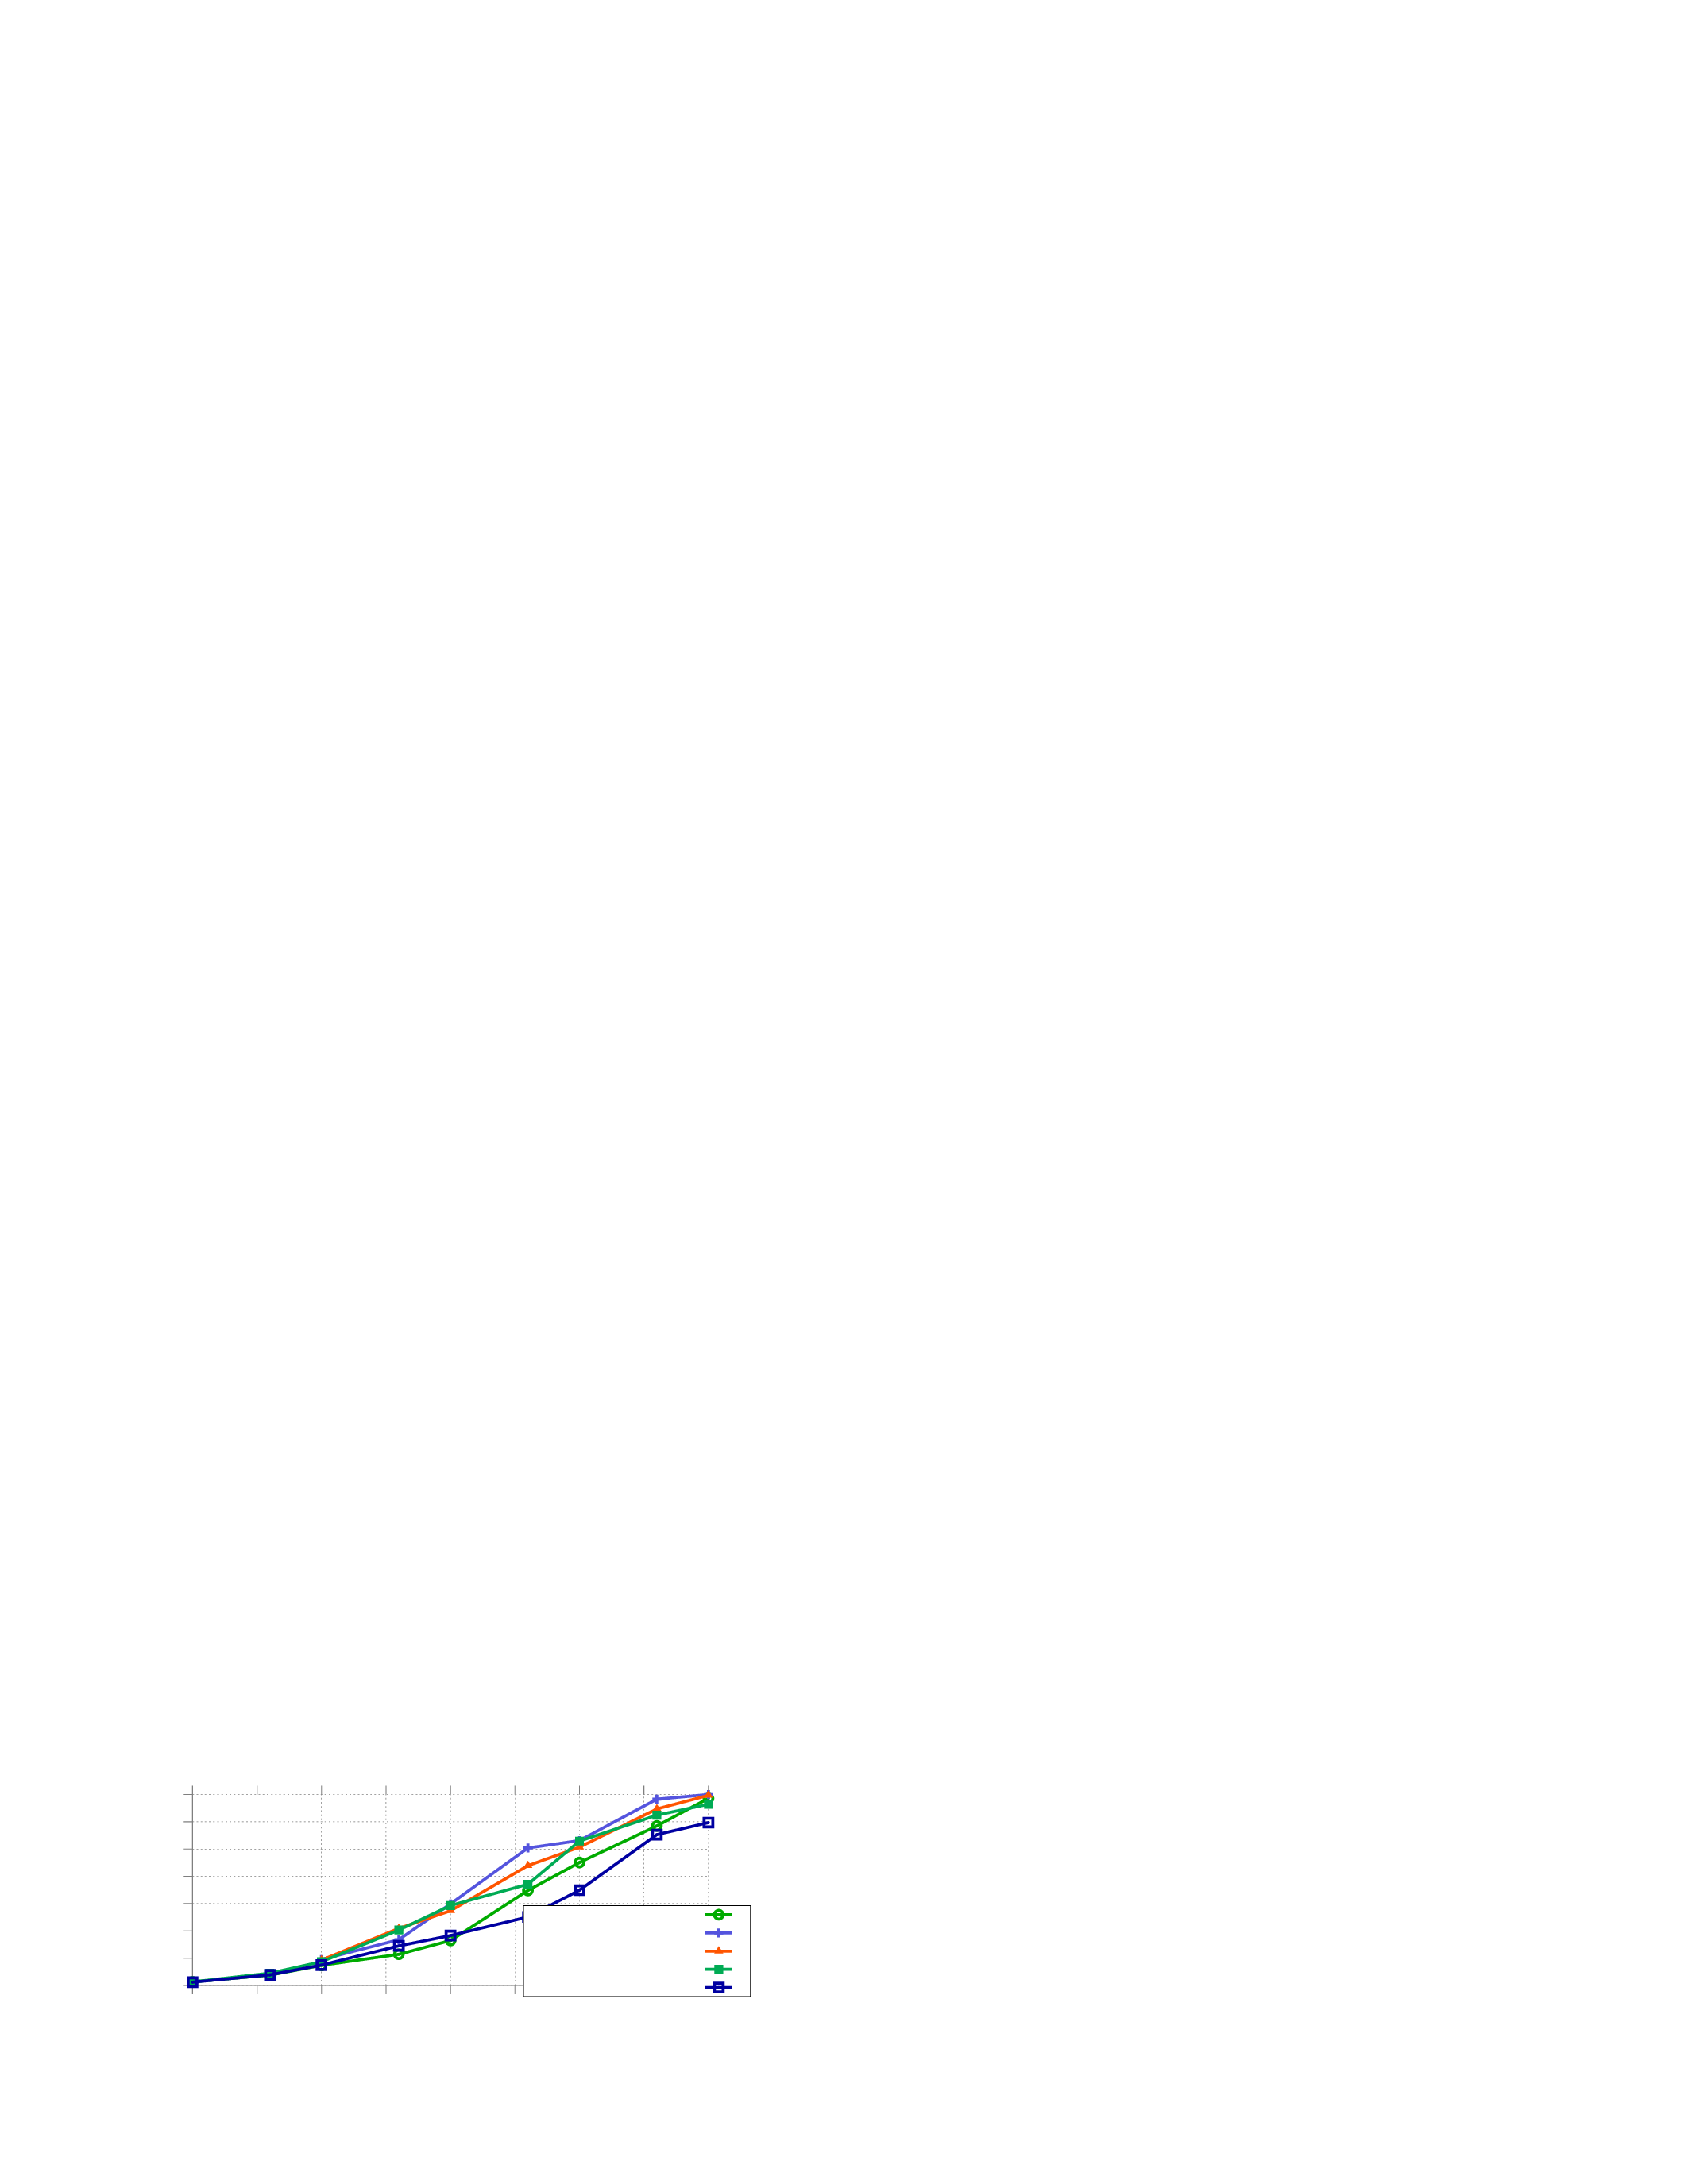}}\label{subfig: fmnist_KL_test}}
	\caption{Comparison on \emph{test data} between the $0-1$ loss obtained by different training methods (computed using AutoAttack) versus the optimal loss.}
	\label{fig: compare_plot_01_test}
	\vspace{-10pt}
\end{figure}

\subsection{Optimal vs. empirical probabilities}

\begin{figure*}[t]
	\centering
	\subfloat[2.0]{\resizebox{0.3\textwidth}{!}{\includegraphics{images/MNIST/3_7_2000_l2_2_0.pdf}}\label{subfig: mnist_2}}
	\subfloat[2.2]{\resizebox{0.3\textwidth}{!}{\includegraphics{images/MNIST/3_7_2000_l2_2_2.pdf}}\label{subfig: mnist_2}}
	\subfloat[2.4]{\resizebox{0.3\textwidth}{!}{\includegraphics{images/MNIST/3_7_2000_l2_2_4.pdf}}\label{subfig: mnist_2}}
	\hspace{0mm}
	\subfloat[2.6]{\resizebox{0.3\textwidth}{!}{\includegraphics{images/MNIST/3_7_2000_l2_2_6.pdf}}\label{subfig: mnist_2}}
	\subfloat[2.8]{\resizebox{0.3\textwidth}{!}{\includegraphics{images/MNIST/3_7_2000_l2_2_8.pdf}}\label{subfig: mnist_2}}
	\subfloat[3.0]{\resizebox{0.3\textwidth}{!}{\includegraphics{images/MNIST/3_7_2000_l2_3_0.pdf}}\label{subfig: mnist_2}}
	\hspace{0mm}
	\subfloat[3.2]{\resizebox{0.3\textwidth}{!}{\includegraphics{images/MNIST/3_7_2000_l2_3_2.pdf}}\label{subfig: mnist_2}}
	\subfloat[3.4]{\resizebox{0.3\textwidth}{!}{\includegraphics{images/MNIST/3_7_2000_l2_3_4.pdf}}\label{subfig: mnist_2}}
	\subfloat[3.6]{\resizebox{0.3\textwidth}{!}{\includegraphics{images/MNIST/3_7_2000_l2_3_6.pdf}}\label{subfig: mnist_2}}
	\hspace{0mm}
	\subfloat[3.8]{\resizebox{0.3\textwidth}{!}{\includegraphics{images/MNIST/3_7_2000_l2_3_8.pdf}}\label{subfig: mnist_2}}
	\subfloat[4.0]{\resizebox{0.3\textwidth}{!}{\includegraphics{images/MNIST/3_7_2000_l2_4_0.pdf}}\label{subfig: mnist_2}}
	\subfloat[4.2]{\resizebox{0.3\textwidth}{!}{\includegraphics{images/MNIST/3_7_2000_l2_4_2.pdf}}\label{subfig: mnist_2}}
	\hspace{0mm}
	\subfloat[4.4]{\resizebox{0.3\textwidth}{!}{\includegraphics{images/MNIST/3_7_2000_l2_4_4.pdf}}\label{subfig: mnist_2}}
	\subfloat[4.6]{\resizebox{0.3\textwidth}{!}{\includegraphics{images/MNIST/3_7_2000_l2_4_6.pdf}}\label{subfig: mnist_2}}
	\subfloat[4.8]{\resizebox{0.3\textwidth}{!}{\includegraphics{images/MNIST/3_7_2000_l2_4_8.pdf}}\label{subfig: mnist_2}}
	%	\subfloat[Fashion MNIST]{\resizebox{0.48\textwidth}{!}{\input{plots/3_7_fmnist_l2_2000_all_.tex}}\label{subfig: fmnist_all_attacks}}
	\caption{Dataset: MNIST. Optimal vs. empirical logloss values.}
	\label{fig: opt_vs_emp_MNIST}
	\vspace{-10pt}
\end{figure*}

\subsection{Further Gaussian results}

\section{More robust training results}

% \subsection{Dropping points}
% \noindent \textbf{Dropping points:} We define a bipartite graph $G'$ over the training data from the two classes based on the composite cost, where an edge exists if $c_N \circ c_N^T(x,x')=0$ and no edge exists otherwise. The vertex set $V_1$ consists of points from class $1$ and $V_{-1}$ of points from class $-1$. The equivalent problem in this setting then becomes that of \emph{maximum cardinality matching}, which is the dual problem to the minimum vertex cover. Further, the complement of the minimum vertex cover is the maximum independent set. The set of points that we need to drop is the minimum vertex cover, since that will remove the most $0$ cost edges, which in turn implies that the classification problem becomes the easiest possible.

% \noindent \textbf{Drop matched points at random.} For each pair of points from opposite classes that is matched at a composite cost of $0$, we drop one of them at random. Since only one of these points can be classified correctly even by the optimal classifier, having both in the training set may hamper convergence if the attack is strong enough. This is validated by our results in the next section.

\subsection{Ablation}

\subsection{CIFAR-10 robust training}
\begin{outline}
	\1 Dropping hard points (doesn't really work, our idea) \todo{Redo experiments with easy points only}
	\1 Using data-based curriculum (doesn't really work, our idea)
	\1 Using benign init (doesn't work at all) \todo{Vikash: qualitative description of observations}
	\1 Using robust init from lower budget (works, closely related to epsilon-scheduling) \todo{Vikash: add the results from robust pre-training}
\end{outline}

\noindent \textbf{Effect of pre-training} To resolve the convergence issues for CIFAR-10 "class 3 vs. 7" classification, we now turn to network pre-training. We find that pre-training with benign cross-entropy loss fails to bring any benefit, even when we use state-of-the-art pretraining techniques~\cite{Kolesnikov2019BigT}. When fine-tuning such a model with robust training, we find that loss quickly increases at the start, an indication of catastrophic forgetting~\cite{kemker2017catforget}. However, we find that robust-pretraining helps in improving the convergence. We pre-train on the full CIFAR-10 dataset with a $\ell_2$ perturbation of 0.5. When fine-tune at $\ell_2$ perturbation of 1.0 on CIFAR-10 "class 3 vs. 7" it achieves 100\% robust accuracy, where without fine-tuning we achieve only 60.4 robust test accuracy. However, it also fails to converge the networks when we fine-tune the model at $\ell_2$ perturbation greater than 3.0.

\subsection{Other class pairs}
